# Supplementary material for: Multiple testing when many $p$-values are uniformly conservative, with application to testing qualitative interaction in educational interventions
Source: arXiv:1703.09787 source file (2017-08-26)
Supplement: Supplementary file 1 [file supplement.tex]

\documentclass[aoas,preprint]{imsart}

\usepackage{cleveref, bm, commath}
\usepackage{graphicx}
\usepackage{subcaption}

\usepackage{natbib}

\usepackage{multirow}
\usepackage{algorithmic}

\usepackage{color}
\definecolor{wjs}{RGB}{0,0,255}

\definecolor{qz}{RGB}{0,255,0}

\usepackage[plain,noend]{algorithm2e}
\usepackage{amsmath, amsfonts, amsthm}

\usepackage{xr}
\externaldocument{paper}

\crefname{assumption}{Assumption}{Assumptions}
\crefname{equation}{equation}{equations}

\theoremstyle{definition}

% \newlength{\dhatheight}
% \newcommand{\doublehat}[1]{%
% \settoheight{\dhatheight}{\ensuremath{\hat{#1}}}%
% \addtolength{\dhatheight}{-0.2ex}%
% \hat{\vphantom{\rule{1pt}{\dhatheight}}%
% \smash{\hat{#1}}}}

% \DeclareMathOperator*{\argmin}{arg\,min}
% \DeclareMathOperator*{\argmax}{arg\,max}

\makeatletter
\renewcommand{\algocf@captiontext}[2]{#1\algocf@typo. \AlCapFnt{}#2} % text of caption
% default definition
\def\@algocf@capt@plain{top}
\renewcommand{\algocf@makecaption}[2]{%
  \addtolength{\hsize}{\algomargin}%
  \sbox\@tempboxa{\algocf@captiontext{#1}{#2}}%
  \ifdim\wd\@tempboxa >\hsize%     % if caption is longer than a line
  \hskip .5\algomargin%
  \parbox[t]{\hsize}{\algocf@captiontext{#1}{#2}}% then caption is not centered
  \else%
  \global\@minipagefalse%
  \hbox to\hsize{\box\@tempboxa}% else caption is centered
  \fi%
  \addtolength{\hsize}{-\algomargin}%
}
\makeatother

\begin{document}

\begin{frontmatter}

\title{Supplement to ``Multiple Testing When Many $p$-values
  are Uniformly Conservative, with application to Qualitative
  Interaction in Educational Intervention''%\protect\thanksref{T1}
}
\runtitle{Supplement}
% \thankstext{T1}{Footnote to the title with the `thankstext' command.}

\end{frontmatter}

\appendix
\input{appendix}

\end{document}
